# Supplementary material for: Reframing Instructional Prompts to GPTk's Language
Source: arXiv:2109.07830 source file (2022-03-15)
Supplement: Supplementary file 1 [file appendix_examples_pattern.tex]

% \begin{table*}[h]
%     \small
%     \centering
%      \resizebox*{!}{0.72\textheight}{%
%     \begin{tabular}{p{16.5cm}}
%         \toprule
%         \textit{Raw task definitions, their \textsc{\textcolor{purple}{Pattern Reframed}} counterparts and GPT3-instruct outputs} \\ 
%         \midrule
%         \textcolor{brown}{\textit{\textbf{Raw Task:}}} \textit{Craft a question which requires commonsense to be answered. Based on the given context, craft a common-sense question, especially those that are LONG, INTERESTING, and COMPLEX. The goal is to write questions that are easy for humans and hard for AI machines! To create such questions, here are some suggestions: A. What may (or may not) be the plausible reason for an event? B. What may (or may not) happen before (or after, or during) an event? C. What may (or may not) be a plausible fact about someone (or something)? D. What may (or may not) happen if an event happens (or did not happen)? You can also create other types of question.} \newline \textbf{Context}:I was told, in person over the phone, that my shoes were on their way. They have my money. I have no shoes. \newline \textbf{Question}: \textcolor{red}{What may be the plausible reason for this event?}\\
%         \cdashlinelr{1-1}
%         \textcolor{brown}{\textit{\textbf{Reframed Task:}}}
%         \textit{Use 'what may happen', 'will ...?', 'why might', 'what may have caused', 'what may be true about', 'what is probably true about', 'what must' and similar phrases in your question based on the input context.}\newline \textbf{Context}:I was told, in person over the phone, that my shoes were on their way. They have my money. I have no shoes. \newline \textbf{Question}:\textcolor{blue}{What may happen if my shoes never show up?}\\ [0.1cm]
%         \midrule
%         \midrule
%         \textcolor{brown}{\textit{\textbf{Raw Task:}}} \textit{Craft a question which requires commonsense to be answered. Based on the given context, craft a common-sense question, especially those that are LONG, INTERESTING, and COMPLEX. The goal is to write questions that are easy for humans and hard for AI machines! To create such questions, here are some suggestions: A. What may (or may not) be the plausible reason for an event? B. What may (or may not) happen before (or after, or during) an event? C. What may (or may not) be a plausible fact about someone (or something)? D. What may (or may not) happen if an event happens (or did not happen)? You can also create other types of question.} \newline \textbf{Context}:you see , at my age relationship is kind of important and i thought i got the one after all these years . I noticed that once again i was wrong . i was good simply because i was good , i was caring , helping , supportive , bla bla blaaa . \newline \textbf{Question}: \textcolor{red}{what is the reason why you keep falling for the same type of person?\newline \newline
%         A. What is the reason you keep falling for the same type of person?\newline
%         B. What may (or may not) be the problem with your relationships?\newline
%         C. What may (or may not) be the possible cause}\\
%         \cdashlinelr{1-1}
%         \textcolor{brown}{\textit{\textbf{Reframed Task:}}}
%         \textit{Use 'what may happen', 'will ...?', 'why might', 'what may have caused', 'what may be true about', 'what is probably true about', 'what must' and similar phrases in your question based on the input context.}\newline \textbf{Context}:you see , at my age relationship is kind of important and i thought i got the one after all these years . I noticed that once again i was wrong . i was good simply because i was good , i was caring , helping , supportive , bla bla blaaa . \newline \textbf{Question}:\textcolor{blue}{What may happen if i don't get the one i want ?}\\ [0.1cm]
%         \midrule
%         \midrule
%         \textcolor{brown}{\textit{\textbf{Raw Task:}}} \textit{Craft a question which requires commonsense to be answered. Based on the given context, craft a common-sense question, especially those that are LONG, INTERESTING, and COMPLEX. The goal is to write questions that are easy for humans and hard for AI machines! To create such questions, here are some suggestions: A. What may (or may not) be the plausible reason for an event? B. What may (or may not) happen before (or after, or during) an event? C. What may (or may not) be a plausible fact about someone (or something)? D. What may (or may not) happen if an event happens (or did not happen)? You can also create other types of question.} \newline \textbf{Context}: GPS technology dates back to the time when first ever satellite was launched in the sky in 1979. The era of global positioning started then. \newline \textbf{Question}: \textcolor{red}{What was the first satellite launched in 1979? \newline \newline
%         A. Voyager 1 \newline
%         B. Voyager 2 \newline
%         C. Pioneer 11 \newline
%         D. Pioneer 10}\\
%         \cdashlinelr{1-1}
%         \textcolor{brown}{\textit{\textbf{Reframed Task:}}}
%         \textit{Use 'what may happen', 'will ...?', 'why might', 'what may have caused', 'what may be true about', 'what is probably true about', 'what must' and similar phrases in your question based on the input context.}\newline \textbf{Context}:GPS technology dates back to the time when first ever satellite was launched in the sky in 1979. The era of global positioning started then. \newline \textbf{Question}:\textcolor{blue}{Why might GPS technology have been invented??}\\
%         \bottomrule
%         \end{tabular}
%         }
%         \caption{
%             Examples of {\bf Pattern Reframed} instructions. 
%             \textit{Italicized} text represents the instructions. 
%             GPT3-instruct's response to the raw and reframed instructions are indicated with \textcolor{blue}{blue} and \textcolor{red}{red} markings, respectively.
%         }
%     \label{tab:pattern_reframing_both1}
% \end{table*}
